# Supplementary material for: Data-Dependent Randomized Smoothing
Source: arXiv:2012.04351 source file (2022-07-05)
Supplement: Supplementary file 3 [file appendix_visualization_cohen.tex]

\captionsetup[subfigure]{labelformat=empty}
\begin{figure}[ht]
\begin{subfigure}{0.16\textwidth}
  \centering
  \includegraphics[width=\textwidth]{ 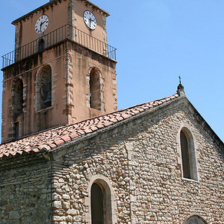}  
  \caption{Clean image}
\end{subfigure}
\begin{subfigure}{0.16\textwidth}
  \centering
  \includegraphics[width=\textwidth]{ 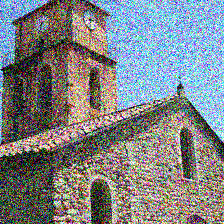} 
  \caption{$\sigma_0 = 0.25$}
\end{subfigure}
\begin{subfigure}{0.16\textwidth}
  \centering
  \includegraphics[width=\textwidth]{ 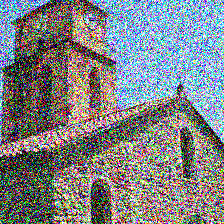}  
  \caption{$\sigma_x^* = 0.392$}
\end{subfigure}
\begin{subfigure}{0.16\textwidth}
  \centering
  \includegraphics[width=\textwidth]{ 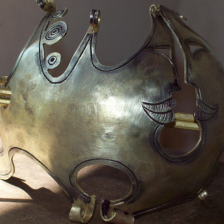}  
  \caption{Clean image}
\end{subfigure}
\begin{subfigure}{0.16\textwidth}
  \centering
  \includegraphics[width=\textwidth]{ 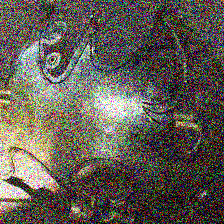} 
  \caption{$\sigma_0 = 0.25$}
\end{subfigure}
\begin{subfigure}{0.16\textwidth}
  \centering
  \includegraphics[width=\textwidth]{ 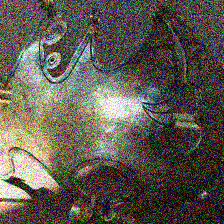}  
  \caption{$\sigma_x^* = 0.169$}
\end{subfigure}
\begin{subfigure}{0.16\textwidth}
  \centering
  \includegraphics[width=\textwidth]{ 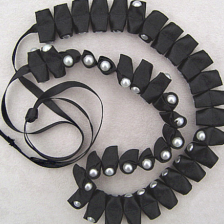}  
  \caption{Clean image}
\end{subfigure}
\begin{subfigure}{0.16\textwidth}
  \centering
  \includegraphics[width=\textwidth]{ 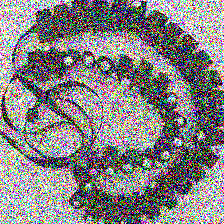} 
  \caption{$\sigma_0 = 0.50$}
\end{subfigure}
\begin{subfigure}{0.16\textwidth}
  \centering
  \includegraphics[width=\textwidth]{ 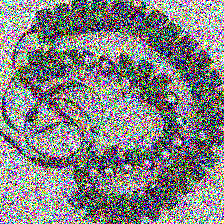}  
  \caption{$\sigma_x^* = 0.705$}
\end{subfigure}
\begin{subfigure}{0.16\textwidth}
  \centering
  \includegraphics[width=\textwidth]{ 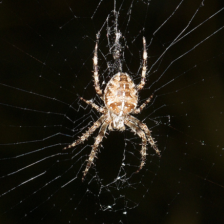}  
  \caption{Clean image}
\end{subfigure}
\begin{subfigure}{0.16\textwidth}
  \centering
  \includegraphics[width=\textwidth]{ 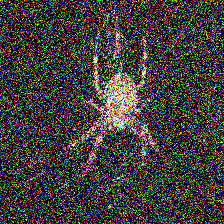} 
  \caption{$\sigma_0 = 0.50$}
\end{subfigure}
\begin{subfigure}{0.16\textwidth}
  \centering
  \includegraphics[width=\textwidth]{ 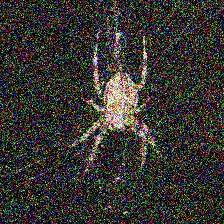}  
  \caption{$\sigma_x^* = 0.368$}
\end{subfigure}
\begin{subfigure}{0.16\textwidth}
  \centering
  \includegraphics[width=\textwidth]{ 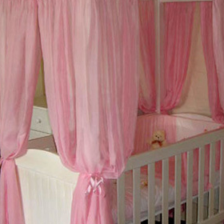}  
  \caption{Clean image}
\end{subfigure}
\begin{subfigure}{0.16\textwidth}
  \centering
  \includegraphics[width=\textwidth]{ 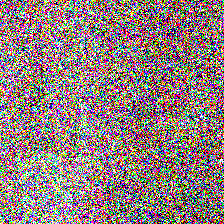} 
  \caption{$\sigma_0 = 1.00$}
\end{subfigure}
\begin{subfigure}{0.16\textwidth}
  \centering
  \includegraphics[width=\textwidth]{ 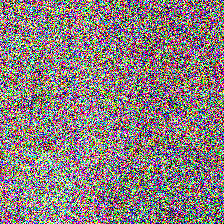}  
  \caption{$\sigma_x^* = 1.267$}
\end{subfigure}
\begin{subfigure}{0.16\textwidth}
  \centering
  \includegraphics[width=\textwidth]{ 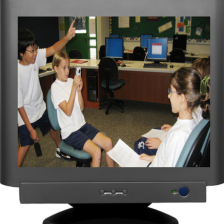}  
  \caption{Clean image}
\end{subfigure}
\begin{subfigure}{0.16\textwidth}
  \centering
  \includegraphics[width=\textwidth]{ 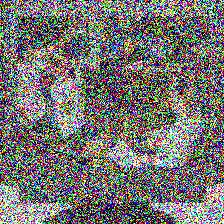} 
  \caption{$\sigma_0 = 1.00$}
\end{subfigure}
\begin{subfigure}{0.16\textwidth}
  \centering
  \includegraphics[width=\textwidth]{ 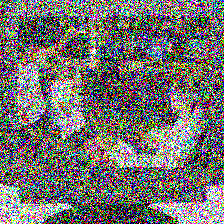}  
  \caption{$\sigma_x^* = 0.813$}
\end{subfigure}\vspace{-0.8cm}
\end{figure}
